# Supplementary material for: Spin-excitation anisotropy in the nematic state of detwinned FeSe
Source: arXiv:2108.04484 source file (2021-12-27)
Supplement: Supplementary file 1 [file Revised_SM_1224.pdf]

# Supplemental Material: Spin-excitation anisotropy in the nematic state of detwinned FeSe

Xingye Lu,\* Wenliang Zhang, Yi Tseng, Ruixian Liu, Zhen Tao, Eugenio Paris, Panpan Liu, Tong Chen, Vladimir Strocov, Yu Song, Rong Yu, Qimiao Si, Pengcheng Dai,<sup>†</sup> and Thorsten Schmitt<sup>‡</sup>  
(Dated: December 24, 2021)

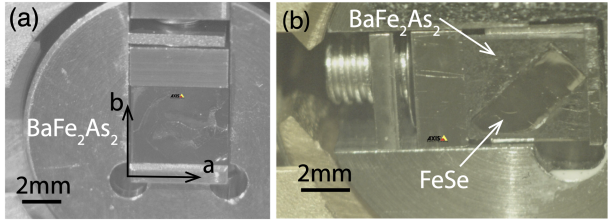

FIG. S1. Mechanical device for detwinning (a) BaFe<sub>2</sub>As<sub>2</sub> and (b) FeSe installed on a RIXS sample holder on SAXES spectrometer at ADDRESS beamline, SLS. Uniaxial pressure is applied via tuning the screw on one end. The pressure can be hold at low temperature by a Belleville spring washer. A large BaFe<sub>2</sub>As<sub>2</sub> crystal ( $5 \times 4.3 \times 0.4 \text{ mm}^3$ ) was inserted into the device in (a) and a FeSe/BaFe<sub>2</sub>As<sub>2</sub> sample in (b). Both samples were cleaved at  $\sim 20 \text{ K}$  in high vacuum ( $\sim 1 \times 10^{-8} \text{ torr}$ ).

## Spin excitation anisotropy and nematic spin correlations

Figure 2 shows how we can connect the spin-excitation anisotropy measured with RIXS to the intrinsic nematic spin correlations. As we have described in the main text, we define the spin-excitation anisotropy as  $\phi(q_{||}) = \frac{\int S_h(q_{||}, E) dE}{\int S_k(q_{||}, E) dE} = S_h(q_{||})/S_k(q_{||})$ , in which  $S_h(q_{||})$  and  $S_k(q_{||})$  are energy integrated spin excitations measured at  $(q_{||}, 0)$  and  $(0, q_{||})$ , respectively. In our previous neutron scattering study, we have defined the nematic spin correlations as  $\psi(E) = \frac{S_1(E) - S_2(E)}{S_1(E) + S_2(E)}$  (or  $\psi(q, E) = \frac{S_1(q, E) - S_2(q, E)}{S_1(q, E) + S_2(q, E)}$ ), where  $S_{1,2}(E) = \frac{\int S_{1,2}(q, E) dq}{\int dq}$ , and the integral  $\int dq$  runs over the whole Brillouin zone (BZ). Note  $q$  is a reduced momentum within a BZ.

As shown in Fig. S2(a), the RIXS spectra  $S_h(q)$  and  $S_k(q)$  measured at  $(q, 0)$  (red dot) and  $(0, q)$  (blue dot) in the first BZ, can be written as:

$$S_h(q) = S_1[(q, 0), E_2] + S_2[(q, 0), E_1] \quad (1)$$

$$S_k(q) = S_1[(0, q), E_1] + S_2[(0, q), E_2] \quad (2)$$

As  $S_h(q) > S_k(q)$  at all the momenta measured, the lower limit for  $\phi(q)$  is 1, which can be realized in a twinned sample, or a system without nematic spin correlations, as shown in Fig. S2(b). The upper limit for  $\phi(q)$  is  $S_1[(q, 0), E_2]/S_1[(0, q), E_1]$ , which can be achieved in a system where  $S_2$  vanishes, such as the Heisenberg model

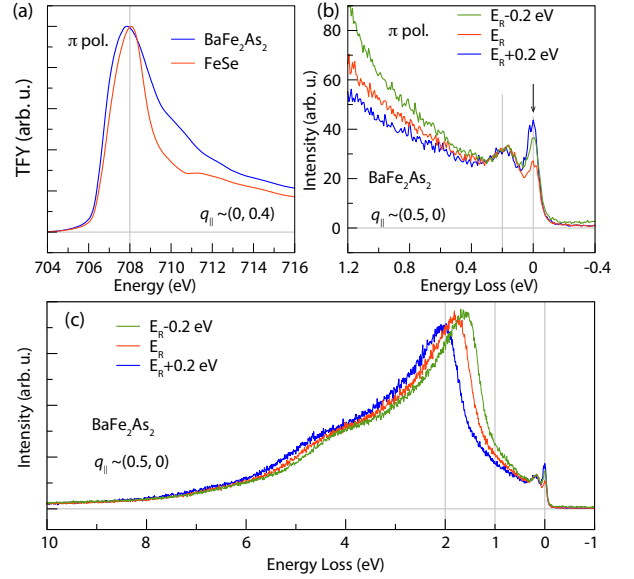

FIG. S2. (a) Comparison of the total fluorescence yield (TFY) XAS spectrum between BaFe<sub>2</sub>As<sub>2</sub> (blue curve) and FeSe (red curve). The Fe- $L_3$  resonance energy ( $E_R$ ) of FeSe is slightly ( $\sim 0.2 \text{ eV}$ ) higher than that for BaFe<sub>2</sub>As<sub>2</sub>. The data were collected at  $q_{||} \sim (0, 0.4)$  and  $T = 20 \text{ K}$  with  $\pi$  polarization. (b),(c) Brief energy detuning RIXS measurements of detwinned BaFe<sub>2</sub>As<sub>2</sub> near the Fe- $L_3$  edge. The measurements were performed at  $T = 20 \text{ K}$  with  $q_{||} = (0.5, 0)$ . The vertical arrow in (b) marks the  $E_i$ -independent spin excitations near the Fe- $L_3$  edge, indicative of its Raman-mode nature. As a comparison, the fluorescence peak (at  $\sim 1.5 - 2 \text{ eV}$ ) in (c) shifts to higher energy with increasing  $E_i$ .

calculation of the intrinsic spin waves in BaFe<sub>2</sub>As<sub>2</sub> [Fig. S2(d)]. Note that the upper limit could be different in BaFe<sub>2</sub>As<sub>2</sub> and FeSe. This could undermine our comparison of the spin-excitation anisotropy between BaFe<sub>2</sub>As<sub>2</sub> and FeSe. For a system with nematic state, the spin-excitation anisotropy  $\phi(q)$  can reflect the amplitude and energy scale of the nematic spin correlations [Fig. S2(c)].

## Fitting of the RIXS spectra

To extract the energy dispersion  $E(q)$ , damping rate, and intensity of the magnetic excitations, we need to use an efficient model to account for the fluorescence ( $I_{\text{flu}}$ ), (para)magnon ( $S(q, E)$ ) and elastic peak ( $I_{\text{el}}$ ) of RIXS

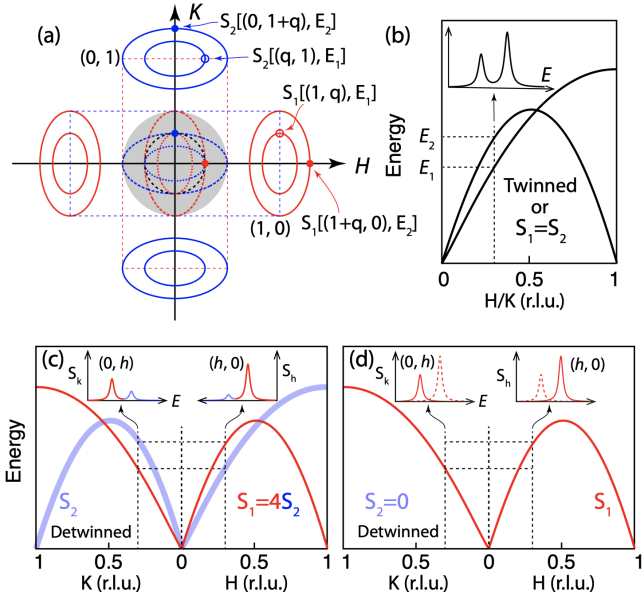

FIG. S3. (a) Reciprocal space and Brillouin zone for typical FeSC systems such as BaFe<sub>2</sub>As<sub>2</sub> and FeSe. The red (blue) dashed rectangle are first BZ centering at  $\Gamma$  point associated with  $Q_1 = (1,0)$  ( $Q_2 = (0,1)$ ). The inner (outer) ellipses mark the constant-energy excitations with an energy transfer of  $E_1$  ( $E_2$ ). (b)-(d) Schematic dispersion for (b) a twinned sample or a sample with no nematic spin correlations ( $S_1 = S_2$ ), (c) a detwinned sample with nematic spin correlations  $S_1 > S_2$ , and (d) a detwinned sample with  $S_1$  only. The insets in (b)-(d) show the corresponding spectra  $S_h$  and  $S_k$ .

spectra. RIXS spectrum at  $q$  can be expressed as:

$$I(E) = I_{\text{fluor}} + S(q, E) + I_{\text{el}} \quad (3)$$

where  $E$  is energy transfer (loss), and  $I_{\text{el}}$  can be described with a resolution-limited gaussian peak. The RIXS spectral weight of iron-based superconductors (FeSC) are usually dominated by strong fluorescence signal at  $E \gtrsim 0.5\text{eV}$ . Accurate description of fluorescence is important for extracting the magnetic scattering. Previous RIXS studies of FeSC have shown that the fluorescence at Fe- $L_3$  edge can be well described by the formula:

$$I_{\text{fluor}} = (bE^2 + aE) \cdot (1 - g_\gamma) + I_0 \exp(-\alpha E) \cdot g_\gamma + G \quad (4)$$

with

$$g_\gamma = \left( \exp\left(\frac{E + E^*}{\Gamma}\right) + 1 \right)^{-1} \quad (5)$$

where  $G = A_0 \exp\left(-\frac{(E + E_s)^2}{2\sigma^2}\right)$  is a gaussian function.  $g_\gamma$  generates a smooth crossover from the quasilinear region with  $E \lesssim 1\text{eV}$  (the first term of Eq. (2)) to the exponential region (the second term of Eq. (2)) [1–3]. As shown in Fig. S2, the overall line-shape of the fluorescence can be well fitted by Eq. (2). Because the magnetic excitations exist only at low energy ( $E \lesssim 0.8\text{eV}$ ), while the

exponential decay dominates the range with much higher energy, we neglect  $g_\gamma$  and describe the low-energy fluorescence using  $bE^2 + aE$  in fitting the magnetic excitations.

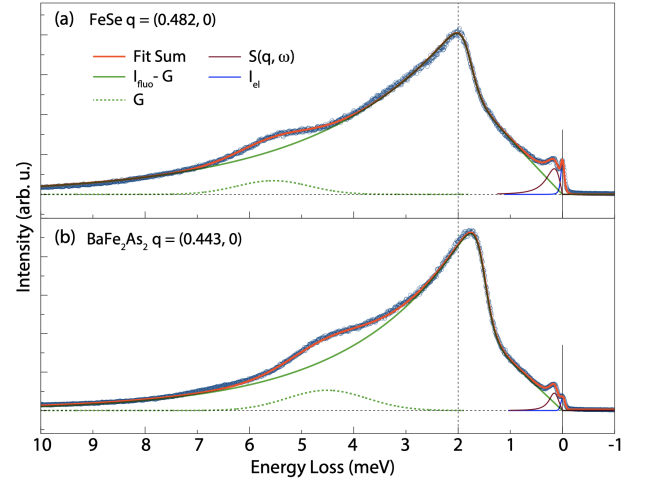

FIG. S4. Fitting of the full RIXS spectra measured at (a)  $q \parallel$

Given that the magnetic excitations are heavily damped in itinerant FeSC, we use a general damped harmonic oscillator function to capture the features of the magnetic excitations [4–7]:

$$S(q, E) = A \frac{E_0}{1 - e^{-\beta E}} \frac{2\gamma E}{(E^2 - E_0^2)^2 + (E\gamma)^2}, \quad (6)$$

where  $\beta$  is  $\frac{1}{k_B T}$  ( $k_B$  is Boltzmann constant).  $E_0(q)$  is the undamped energy and  $\gamma(q)$  the excitation life time (which represents the damping rate). When the excitations are underdamped ( $\gamma/2 < E_0$ ), we can also describe the spectrum using an antisymmetrized Lorentzian function [5–7],

$$S(q, E) \propto \frac{\gamma/2}{(E - E_q)^2 + (\gamma/2)^2} + \frac{\gamma/2}{(E + E_q)^2 + (\gamma/2)^2}, \quad (7)$$

generating the fitted pole energies  $E_q = [E_0^2 - (\gamma/2)^2]^{-1/2}$ . In a general case, the undamped energy  $E_0$  and the excitation life time  $\gamma$  are essential information we need to extract from the fitting of the spectra.

We show in Fig. S4 the overall fitting of the RIXS spectra (blue open circles) using Eq. (1) (red curves), and in Figs. S5 and S6 the fitting of the low-energy magnetic excitations for BaFe<sub>2</sub>As<sub>2</sub> and FeSe using Eq. (4). The spectra are well fitted by the damped harmonic oscillator model. The energy dispersions and integrated intensities for BaFe<sub>2</sub>As<sub>2</sub> and FeSe have been shown in the main text.

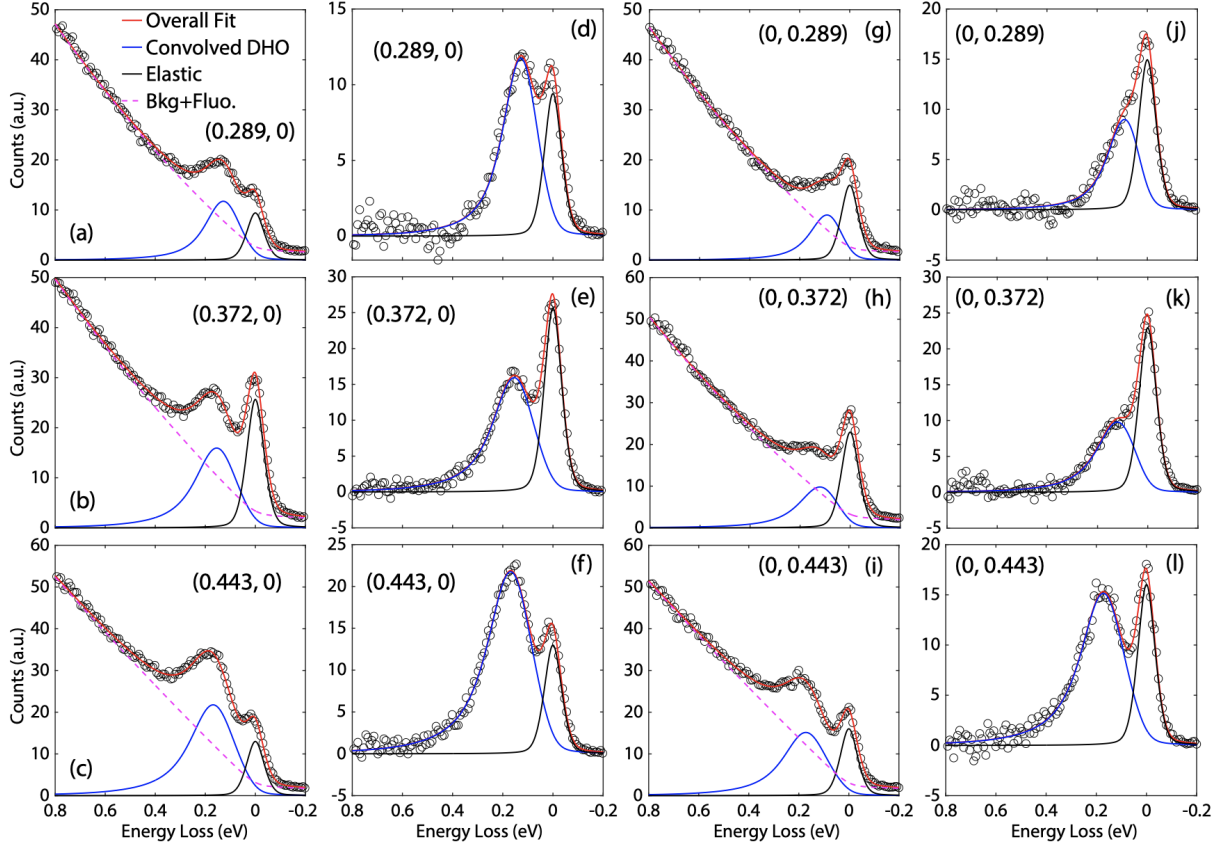

FIG. S5. Selected RIXS spectra along  $[H, 0]$  and  $[0, K]$  directions for detwinned  $\text{BaFe}_2\text{As}_2$  and their fittings using the model as described in Eq. (1). Black circles in (a)-(c), (g)-(i) are raw RIXS spectra, and in (d)-(f), (j)-(l) are spectra with fluorescence and background subtracted. Blue curves are damped harmonic oscillator (DHO) model convolved with an energy-resolution limited gaussian. Black curves are gaussian fittings of the elastic scattering peaks. Pink dashed curves are fluorescence and background. Red curves are overall fit of the spectra.

### Theoretical results

Motivated by the dispersive and underdamped feature of the RIXS spectrum in the detwinned  $\text{FeSe}$ , we study the spin dynamics of an  $S = 1$  bilinear-biquadratic Heisenberg model. The Hamiltonian reads

$$H = \frac{1}{2} \sum_{i, \delta_n, \alpha, \beta} \{J_n \mathbf{S}_i \cdot \mathbf{S}_j + K_n (\mathbf{S}_i \cdot \mathbf{S}_j)^2\}, \quad (8)$$

where  $j = i + \delta_n$ , and  $\delta_n$  connects a site  $i$  in a square lattice and its  $n$ 's nearest neighbor sites with  $n = 1, 2, 3$ . Here  $J_n$ , and  $K_n$  are respectively the bilinear and biquadratic couplings between the  $n$ 's nearest neighbor spins. Unlike  $\text{BaFe}_2\text{As}_2$ , the ground state of  $\text{FeSe}$  is not magnetically ordered but can hold an antiferroquadrupolar (AFQ) order with wave vector  $(\pi, 0)$  [8].

Following this, we study the spin dynamics through Schwinger bosons in an  $SU(3)$  representation [10]. At each site, we use  $|-1\rangle$ ,  $|0\rangle$ , and  $|1\rangle$  to denote the three eigenstates of the spin operator  $S^z$ . They are used for a

time-reversal invariant basis of the  $SU(3)$  representation:

$$\begin{aligned} |x\rangle &= \frac{i}{\sqrt{2}} (|1\rangle - |-1\rangle), \\ |y\rangle &= \frac{1}{\sqrt{2}} (|1\rangle + |-1\rangle), \\ |z\rangle &= -i|0\rangle. \end{aligned} \quad (9)$$

Within this representation, three Schwinger bosons are associated with the three states,  $b_\alpha^\dagger |\emptyset\rangle = |\alpha\rangle$ , where  $\alpha = x, y, z$ , and  $|\emptyset\rangle$  is the null state of the Schwinger bosons. The bosons satisfy a local constraint at each site:

$$\sum_\alpha b_{i\alpha}^\dagger b_{i\alpha} = 1. \quad (10)$$

The spin dipolar and quadrupolar operators can be writ-

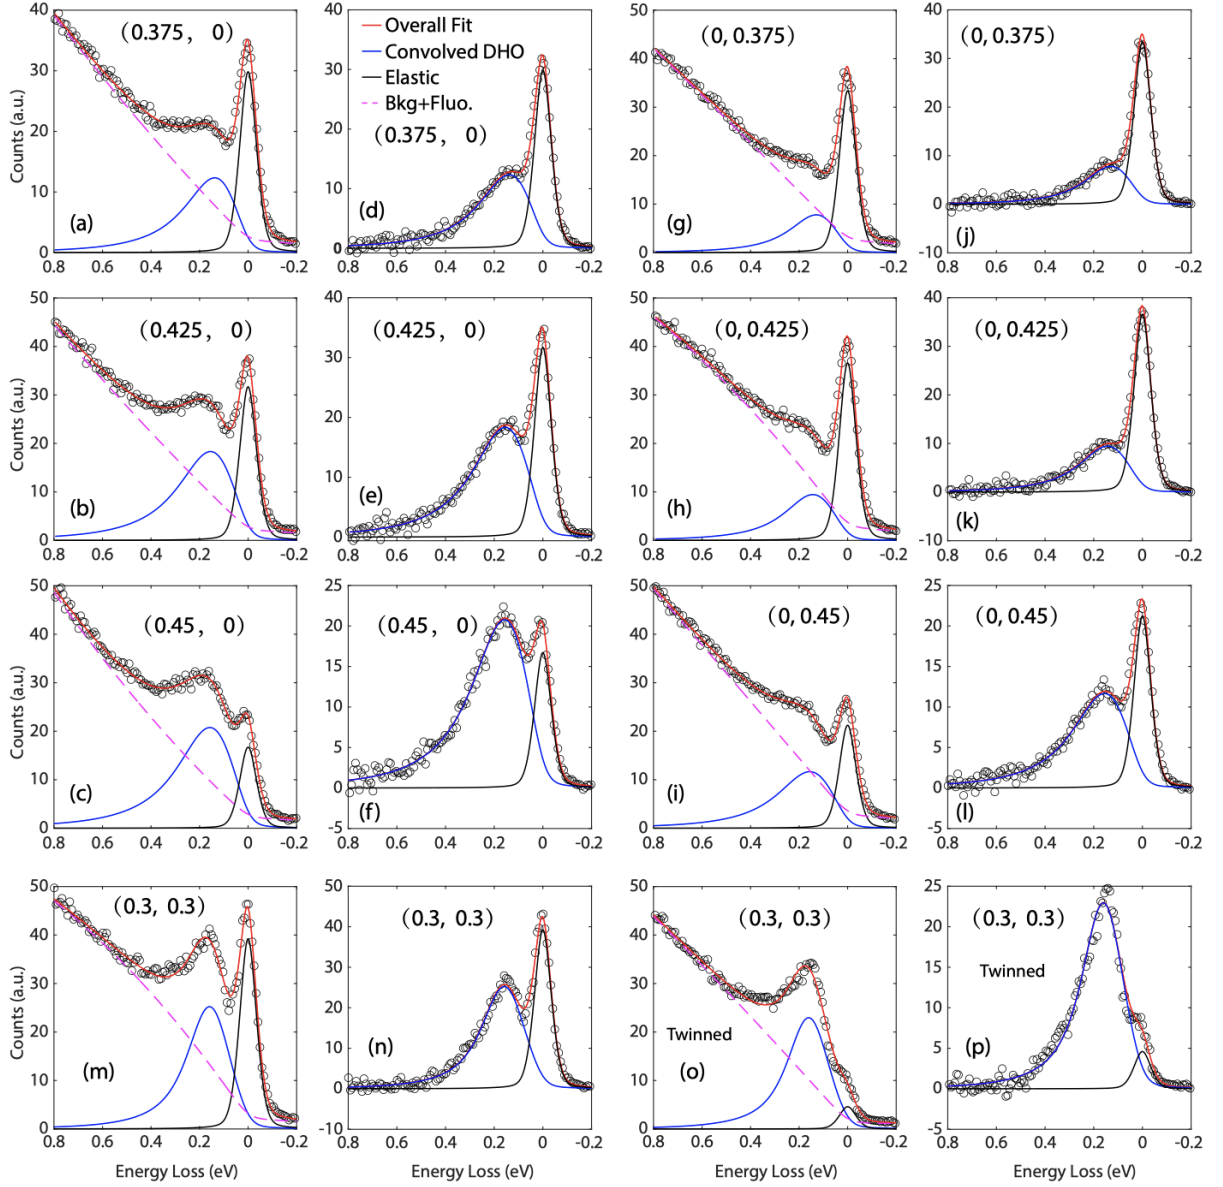

FIG. S6. Fitting of the RIXS spectra of FeSe following the same procedure as that for  $\text{BaFe}_2\text{As}_2$  in Fig. 3. The spectra in (o) and (p) are measured on twinned sample while the others on detwinned sample.

ten in terms of the Schwinger boson bilinears as

$$S_i^\alpha = -i\epsilon_{\alpha\beta\gamma}(b_{i\beta}^\dagger b_{i\gamma} - b_{i\gamma}^\dagger b_{i\beta}), \quad (11)$$

$$\begin{aligned} Q_i^{\alpha\beta} &= -(b_{i\alpha}^\dagger b_{i\beta} + b_{i\beta}^\dagger b_{i\alpha}), \\ Q_i^{x^2-y^2} &= -(b_{ix}^\dagger b_{ix} - b_{iy}^\dagger b_{iy}), \\ Q_i^{x^2-3z^2} &= \frac{1}{\sqrt{3}}(2b_{iz}^\dagger b_{iz} - b_{ix}^\dagger b_{ix} - b_{iy}^\dagger b_{iy}), \end{aligned} \quad (12)$$

where  $\alpha, \beta$ , and  $\gamma$  run over  $x, y$ , and  $z$ , and  $\epsilon_{\alpha\beta\gamma}$  is the Levi-Civita symbol. The Hamiltonian can be rewritten in terms of these Schwinger bosons. The condensation of the boson(s) describes a quadrupolar order. We focus on

condensing the  $b_x$  and  $b_y$  bosons in alternating columns, which specifies the  $(\pi, 0)$  AFQ order of the  $Q^{x^2-y^2}$  type.

We study the spin excitations in the AFQ phase by using the flavor-wave theory. Referring the detail of the calculation to Ref. [8, 9], here we outline the main results. The transverse dynamical spin structure factor is given as follows:

$$S_D^{xx}(\mathbf{q}, \omega) = \frac{1}{2} \sqrt{\frac{A_{\mathbf{q}} + B_{\mathbf{q}}}{A_{\mathbf{q}} - B_{\mathbf{q}}}} \delta(\omega - \epsilon_{\mathbf{q}}), \quad (13)$$

where the magnetic excitation spectrum is

$$\epsilon_{\mathbf{q}} = \sqrt{A_{\mathbf{q}}^2 - B_{\mathbf{q}}^2}, \quad (14)$$

$$A_{\mathbf{q}} = J_1 \cos q_y + J_3(\cos 2q_x + \cos 2q_y) - K_1 - 2K_3, \quad (15)$$

$$B_{\mathbf{q}} = (K_1 - J_1) \cos q_y + (K_3 - J_3)(\cos 2q_x + \cos 2q_y). \quad (16)$$

The dispersion of the magnetic excitations for the parameter set  $J_1 = J_2 = 10$  meV,  $J_3 = -20$  meV,  $K_1 = -28$  meV,  $K_2 = 48$  meV, and  $K_3 = -68$  meV are shown in Fig. 5(a) of the main text. It signals a Goldstone mode at the Brillouin zone center and exhibits anisotropy along the [H,0] (red line) and [0,H] (blue line) directions. We have made no effort to fine-tune the model parameters, and the theoretical dispersion already provides a good description of the experimental data taking into account the size of the experimental resolution (about 80 meV). Because the dispersion of the transverse excitations does not depend on  $J_2$  and  $K_2$  and also due to the size of the experimental error bar, the model parameters cannot be fully determined by fitting the experimental data.

We further calculate the dynamical spin structure factor along several high symmetric directions of the Brillouin zone. The results along the [H,0], [0,H], and [H,H] directions are presented in Fig. 5(b) and (c) of the main text. We have adopted a phenomenological damping parameter  $\gamma$  in the calculation, and take  $\gamma/2 = 100$  meV,  $\gamma/2 = 150$  meV, and  $\gamma/2 = 125$  meV along the [H,0], [0,H], and [H,H] directions, respectively (indicated as the error bars in Fig. 5(a)). By comparing the spectral weights along the [H,0] and [0,H] directions we find an increasing spectral weight anisotropy with increasing momentum transfer. This anisotropic feature is inherent in the coherence factor of  $S_D^{xx}(\mathbf{q}, \omega)$  in Eq. (13).

In summary, we have found that both the spectral weight anisotropy and the dispersion of excitations agree well with experimental results. From this, we can infer that well-defined collective magnetic excitations exist up

to about 200 meV in FeSe. The calculated magnetic excitations are associated with the  $(\pi, 0)$  AFQ order, which arise from a model of quasi-localized magnetic moments with frustrated exchange interactions. Our results further highlight the important role of strong electron correlations in FeSe and related iron-based superconductors.

---

\* luxy@bnu.edu.cn

† pdai@rice.edu

‡ thorsten.schmitt@psi.ch

- [1] Zhou, K. *et al.*, *Persistent high-energy spin excitations in iron-pnictide superconductors*. Nat. Commun. **4**, 1470 (2013).
- [2] Pelliciani *et al.*, *Local and collective magnetism of EuFe<sub>2</sub>As<sub>2</sub>*. Phys. Rev. B **95**, 115152 (2017).
- [3] Hancock, J. N. *et al.*, *Evidence for core-hole-mediated inelastic x-ray scattering from metallic Fe<sub>1.087</sub>Te*. Phys. Rev. B **82**, 020513(R) (2010).
- [4] Lamsal, J. *et al.*, *Extracting paramagnon excitations from resonant inelastic x-ray scattering experiments*. Phys. Rev. B **93**, 214513 (2016).
- [5] Monney, C. *et al.*, *Resonant inelastic x-ray scattering study of the spin and charge excitations in the overdoped superconductor La<sub>1.77</sub>Sr<sub>0.23</sub>CuO<sub>4</sub>*. Phys. Rev. B **93**, 075103 (2016).
- [6] Peng, Y. Y. *et al.*, *Dispersion, damping, and intensity of spin excitations in the monolayer (Bi,Pb)<sub>2</sub>(Sr,La)<sub>2</sub>CuO<sub>6+δ</sub> cuprate superconductor family*. Phys. Rev. B **98**, 144507 (2018).
- [7] Rahn, M. C. *et al.*, *Paramagnon dispersion in β-FeSe observed by Fe L-edge resonant inelastic x-ray scattering*. Phys. Rev. B **99**, 014505 (2019).
- [8] Yu, R. & Si, Q., *Antiferroquadrupolar and Ising-nematic orders of a frustrated bilinear-biquadratic Heisenberg model and implications for the magnetism of FeSe*. Phys. Rev. Lett. **115**, 116401 (2015).
- [9] Lai, H.-H., Hu, W. J., Nica, E. M., Yu, Rong & Si, Q., *Antiferroquadrupolar order and rotational symmetry breaking in a generalized bilinear-biquadratic model on a square lattice*. Phys. Rev. Lett. **118**, 176401 (2017).
- [10] Läuchli, A., Mila, F. & Penc, K., *Quadrupolar Phases of the S = 1 Bilinear-Biquadratic Heisenberg Model on the Triangular Lattice*. Phys. Rev. Lett. **97**, 087205 (2006).
